# Supplementary material for: Beyond Background Shift: Rethinking Instance Replay in Continual Semantic Segmentation
Source: arXiv:2503.22136 source file (2025-03-28)
Supplement: Supplementary file 1 [file X_suppl.tex]

\clearpage
\setcounter{page}{1}
\maketitlesupplementary

\section{Supplementary Experiments}

In this section, we provide an extensive and comprehensive display of experiments. We have structured this section into three subsections. The initial subsection focuses on conducting a sensitivity analysis of the hyper-parameters mentioned in the main paper.  Secondly, we analyze the background shift problem. In the following subsection, we further analyze the effectiveness of our method. Lastly, we provide an in-depth analysis of the state-of-the-art comparison experiments outlined in the main paper.

\subsection{Sensitivity Analysis of Hyper-parameters}

% 在下面这个section中，我们展示了 memory size, the number of instances placed on each image 的消融实验分析。we present the analysis of ablation experiments examining the impact of memory size and the number of instances placed on each image.

%aim to investigate the impact of different components in our method.
% In this section, we present the analysis of ablation experiments examining the impact of memory size, the number of instances placed on each image, the region number, the instance size, the fusion strategy and the mixup strategy.

In this section, we present the analysis of ablation experiments examining the impact of different components in our method.

\noindent
{\bf Sensitivity Analysis of Memory Size~~}
In Figure~\ref{fig: instance_num}, we present a comparative analysis of experiments conducted with varying quantities of stored instances. As illustrated, the performance of the model improves across old classes, new classes, and overall as the number of stored instances increases. Notably, the improvement in performance for new classes is significantly greater than that for old classes, indicating that our instance replay method effectively mitigates forgetting while enhancing the model’s ability to learn new classes. Furthermore, once the number of stored instances reaches a certain threshold, the performance gains begin to stabilize.

\begin{figure}[H]
    % \caption{mIoU on VOC 5-3 with different instance number.}
    \centering
    \includegraphics[width=1\linewidth]{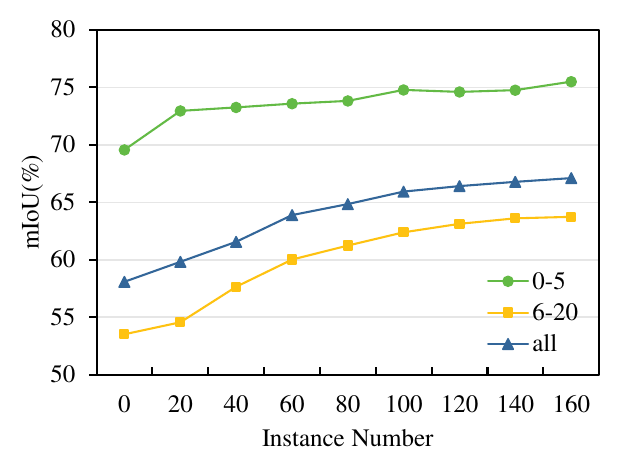}
    \vspace{-0.3in}
    \caption{mIoU on VOC 5-3 with different instance number.}
    \label{fig: instance_num}
\end{figure}

\begin{table}[t]
  \centering
  \caption{The results of sensitivity analysis of instance fusion number on the Pascal VOC 2012 on 5-3 overlapped setting.}

    \vspace{-0.1in}
   \begin{tabular}{c|ccc}
    \Xhline{1.3pt}
      \multirow{1}*{Instance Number} & 0-5 & 6-20 & all\\
      \hline
      % 0& 74.59& 53.16 & 58.28\\ 
       1& 73.83 & 63.10 &66.17 \\ 
       2&\textbf{ 74.61} & \textbf{63.13}& \textbf{66.41}\\
       3&  75.33& 61.32 & 65.32 \\ 
       4& 72.95 & 59.10& 63.06 \\ 
    \Xhline{1.3pt}
    \end{tabular}
    \label{fusion-number}
    % \caption{Instance Fusion Number on the Pascal VOC 2012 5-3 overlapped setting.}
    \vspace{-0.1in}
\end{table}

\noindent
{\bf Sensitivity Analysis of Instance Fusion Number~~}
To analyze the effects of the number of fused instances within each image, we varied the number within \(\left \{ 0,1,2,3,4 \right \}\). As shown in Table~\ref{fusion-number}, under the 5-3 setting on Pascal VOC 2012, the results demonstrate that not fusing any instances leads to severe catastrophic forgetting. The best performance is observed when two instances are fused per image, while fusing as many as four instances negatively impacts the learning of new classes. We think this is because of the over-presentation of old classes within a single image, which creates an imbalance between new and old classes and biases the model's learning toward the old ones. Therefore, we have empirically set the number of fused instances to 2 per image for all experiments.

\begin{table}[t]
  \centering
  \caption{The results of sensitivity analysis of region number on the Pascal VOC 2012 on 5-3 overlapped setting.}

    \vspace{-0.1in}
   \begin{tabular}{c|ccc}
    \Xhline{1.3pt}
      \multirow{1}*{Region Number} & 0-5 & 6-20 & all\\
      \hline
       4& 74.26 & 61.90 & 65.43\\ 
       6& \textbf{74.61} & \textbf{63.13} & \textbf{66.41}\\ 
       9& 73.63 & 61.83 & 65.20\\ 
       12& 73.51 & 61.48 & 64.92\\
    \Xhline{1.3pt}
    \end{tabular}
    \label{region-number}
    % \caption{Instance Fusion Number on the Pascal VOC 2012 5-3 overlapped setting.}
    \vspace{-0.1in}
\end{table}

\noindent
{\bf Sensitivity Analysis of Region Number~~} In the instance placement section, we divide the new image into n regions and specifically selected a portion with a higher proportion of background pixels. Therefore, we varied the \(n\) within \(\left \{ 4,6,9,12 \right \}\) to analyze the effects of region number. The experimental results are compiled into Table~\ref{region-number}. The best performance is observed when the number of regions is divided into \(6\), while increasing or decreasing the number of regions has a negative impact on the learning of new classes. Therefore, we think that a region count of six is more conducive to identifying background areas, thereby enhancing the effectiveness of mitigating background shift issue.

\noindent
{\bf Sensitivity Analysis of Instance Size~~} In Table~\ref{tab: instance-size}, we conducted comprehensive ablation experiments on the size of instances to explore its specific impact on experimental results. Here, we compared three strategies: (1) Original Size (Cropping Excess): maintaining the original size of the instance and cropped any portions exceeding the image boundaries. (2) Adaptively Adjusted to Fit within Image: adjusting the size of the instance to ensure it fit completely within the region in the image without any cropping or overflow. (3) Randomly Enlarge or Shrink: randomly adjusting the size of the instance by selecting a random number from the interval [0,2] and using it as a multiplier to either increase or decrease the dimensions of the instance. The experimental results indicate that strategy (2) yield the optimal results. We think the inefficacy of the original size strategy to the potential omission of crucial information from instances due to cropping beyond image boundaries, which is vital for the experimental results. Moreover, randomly resizing the instances may lead to significant variations in their dimensions, and this inconsistency in size could potentially disrupt the model's training process.

%实验结果显示，策略(2)取得了最佳效果。我们认为，原始大小策略效果不佳的原因在于，裁剪超出图像边界的部分可能会剔除实例的关键信息，这些信息对实验结果具有重要影响。另一方面，随机调整实例大小则可能导致各实例间尺寸差异显著，这种尺寸上的不一致性可能会扰乱模型的训练。

\begin{table}[t]
    \centering
    % \vspace{-0.20in}
    \caption{Results of different size of instance. The performance is reported on Pascal VOC 5-3 overlapped setting.}

    \vspace{-0.1in}
    \begin{tabular}{c|ccc}
    \Xhline{1.3pt}
    \multirow{1}*{Method} & 0-5 & 6-20 & all\\
    \hline
    Original Size    &  73.90 & 60.49 & 64.32\\ 
    Adjusted to Fit Image  &{\bf 74.61} & {\bf 63.13} & {\bf 66.41}\\ 
    Randomly Enlarge or Shrink &72.47 & 60.26 & 63.75 \\ 
    \Xhline{1.3pt}
    \end{tabular}
    \vspace{-0.2in}
    \label{tab: instance-size}   
    % \vspace{-0.05in}
\end{table}

% 怎样贴的消融实验  mixup & 其他的方式  这个是之前aaai中的实验，但是要再想一个方法
%① mixup   ②copy-paste  ③ 
\noindent
{\bf Sensitivity Analysis of Fusion Strategy~~} In Table~\ref{tab: fusion}, we also investigate the impact of different strategies for replaying old class instances in the training data background on model performance. Here, we compare three instance augmentation strategies: (1) Masaike: combining multiple instances within a single image, placing each instance distinctly in its own quadrant; (2) Copy-Paste: directly copying and pasting instances into the background of new data; (3) Mixup: employing mixup technique to fuse instances into the background of new data. The comparison between ``Copy-Paste'' and  ``Mixup'' reflects that the mixup method can enhance the model's plasticity. Additionally, we observed that while the overall performance of the copy-paste method is better than no-replay, the performance for old classes is inferior. This supports our previous assertion that random instance replay can potentially lead to negative impacts and further underscores the necessity of using the mixup method to ensure model stability and effectiveness.

\begin{table}[t]
    \centering
    \vspace{0.1in}
    \caption{Results of different fusion methods. The performance is reported on Pascal VOC 5-3 overlapped setting.}
    \vspace{-0.1in}

    % \vspace{-0.1in}
    \begin{tabular}{c|ccc}
    \Xhline{1.3pt}
    \multirow{1}*{Method} & 0-5 & 6-20 & all\\
    \hline
      Masaike & 60.86 & 56.80 & 57.96\\ 
      Copy-Paste & 72.60 & 59.69 & 63.38\\ 
      Mixup& {\bf 74.61} & {\bf 63.13} & {\bf 66.41}\\ 
    \Xhline{1.3pt}
    \end{tabular}
    \vspace{-0.1in}
    \label{tab: fusion}   
    % \vspace{-0.05in}
\end{table}

%还有一组没有做
% mixup的参数的消融实验
%在将实例融入图像的过程中，我们采用了mixup技术，以确保旧类实例能够自然地融合到新图像的背景中。为了深入探究mixup技术中参数λ的影响，我们设计了一系列消融实验，具体设置如下：①基于beta分布动态选择λ值；②将λ固定为0.2；③将λ固定为0.4；④将λ固定为0.6；⑤将λ固定为0.8。
%我们发现为λ设置固定的值的实验结果 没有 基于beta分布中动态选择的实验结果高，因此 动态选择这种方式更有利于 将instance更自然地融入到新图像中，促进新旧类地学习。
\noindent
{\bf Sensitivity Analysis of Mixup ~~} During the process of integrating instances into images, we employ the mixup technique to ensure that instances seamlessly integrate into the new image. To thoroughly investigate the impact of the parameter \(\lambda \) in the mixup technique, we devise a series of ablation experiments with the following specific settings: (1) dynamically selecting \(\lambda\) based on beta distribution; (2) fixing \(\lambda \) at 0.2; (3) fixing \(\lambda \) at 0.4; (4) fixing \(\lambda \) at 0.6; and (5) fixing \(\lambda \) at 0.8. The experimental results are compiled into Table~\ref{tab: mixup} for analysis. We find that the experimental results obtained by setting a fixed value for \(\lambda \) are not as high as those achieved through dynamic selection based on a beta distribution. Therefore, this dynamic selection method is more conducive to naturally integrating instances into new images, facilitating the learning of both old and new classes.

\begin{table}[t]
    \centering
    % \vspace{-0.20in}
    \caption{Results of different \(\lambda \) in mixup. The performance is reported on Pascal VOC 5-3 overlapped setting.}

    \vspace{-0.1in}
    \begin{tabular}{c|ccc}
    \Xhline{1.3pt}
    \multirow{1}*{Method} & 0-5 & 6-20 & all\\
    \hline
     Beta distrib. &{\bf 74.61} & {\bf 63.13} & {\bf 66.41}\\ 
       0.2 & 72.54 & 61.44 & 64.61\\ 
       0.4 & 71.30 & 59.79 & 63.08\\ 
       0.6 & 73.48 & 61.16 & 64.68\\ 
       0.8 & 74.79 & 62.08 & 65.71\\  
    \Xhline{1.3pt}
    \end{tabular}
    \vspace{-0.2in}
    \label{tab: mixup}   
     \vspace{0.05in}
\end{table}

\begin{table*}[t]
    \centering
    \caption{Experimental results on Pascal VOC 2012 for overlap setting using Resnet101}

    \vspace{-0.1in}
    \begin{tabular}{c|ccc|ccc|ccc|ccc}
    \Xhline{1.3pt}
    \multirow{2}*{\textbf{Method}} & \multicolumn{3}{c|}{\textbf{VOC 10-1} (11)}&\multicolumn{3}{c|}{\textbf{VOC 15-1} (6)}& \multicolumn{3}{c|}{\textbf{VOC 5-3} (6)}& \multicolumn{3}{c}{\textbf{VOC 15-5} (2)}\\ 
    \multicolumn{1}{c|}{} & 0-10 & 11-20 & all & 0-15 & 16-20 & all & 0-5& 6-20& all & 0-15 & 16-20 & all \\
    \hline
    \hline
 MicroSeg-M\cite{zhang2022mining}&  73.1& 52.9& 63.5& 80.4& 42.2& 71.3& 73.5& 60.3& 64.1& 81.5& 55.0&75.2\\
     \hline
     Microseg-EIR& \textbf{74.3}& \textbf{55.0} &\textbf{ 65.1} & {\bf 82.7}& {\bf 55.9}& {\bf 76.3}&\textbf{ 79.9}& \textbf{62.5}&\textbf{67.5} &{\bf 82.5}&{\bf 62.0}&{\bf 77.6}\\
    \Xhline{1.3pt}
    \end{tabular}
    \label{table3}
    \label{tab: contrast}
    \vspace{-0.05in}
\end{table*}

% \begin{table*}[t]
%     \centering
%     \caption{Experimental results on Pascal VOC 2012 for overlap setting using Resnet101}
%     \renewcommand\tabcolsep{4.5pt}
%     \renewcommand{\arraystretch}{1.1}
%     \vspace{-0.1in}
%     \begin{tabular}{c|ccc|ccc|ccc|ccc|ccc}
%     \Xhline{1.3pt}
%     \multirow{2}*{\textbf{Method}} & \multicolumn{3}{c|}{\textbf{VOC 10-1} (11)}&\multicolumn{3}{c|}{\textbf{VOC 15-1} (6)}& \multicolumn{3}{c|}{\textbf{VOC 5-3} (6)}& \multicolumn{3}{c|}{\textbf{VOC 2-2} (10)} & \multicolumn{3}{c}{\textbf{VOC 15-5} (2)}\\ 
%     \multicolumn{1}{c|}{} & 0-10 & 11-20 & all & 0-15 & 16-20 & all & 0-2& 3-20& all & 0-2 & 3-20 & all & 0-15 & 16-20 & all \\
%     \hline
%     \hline
%  MicroSeg-M\cite{zhang2022mining}&  73.1& 52.9& 63.5& 80.4& 42.2& 71.3& 73.5& 60.3& 64.1& 59.4& 46.7& 48.5& 81.5& 55.0&75.2\\
%      \hline
%      Microseg-EIR& \textbf{74.3}& \textbf{55.0} &\textbf{ 65.1} & {\bf 82.7}& {\bf 55.9}& {\bf 76.3}&\textbf{ 79.9}& \textbf{62.5}&\textbf{67.5} & \textbf{60.2}  & \textbf{48.7 }& \textbf{50.3} &{\bf 82.51}&{\bf 62.01}&{\bf 77.63}\\
%     \Xhline{1.3pt}
%     \end{tabular}
%     \label{table3}
%     \label{tab: contrast}
%     \vspace{-0.05in}
% \end{table*}

\begin{table*}[t]
    \centering

    \caption{Experimental results on Pascal VOC 2012 for \textit{disjoint} setup using Resnet101}
    \vspace{-0.1in}
    \begin{tabular}{c|ccc|ccc|ccc|ccc}
    \Xhline{1.3pt}
    \multirow{2}*{\textbf{Method}} & \multicolumn{3}{c|}{\textbf{VOC 10-1} (11)}&\multicolumn{3}{c|}{\textbf{VOC 15-1} (6)}& \multicolumn{3}{c|}{\textbf{VOC 19-1} (2)}& \multicolumn{3}{c}{\textbf{VOC 15-5} (2)}\\
    
    \multicolumn{1}{c|}{}& 0-10 & 11-20 & all & 0-15 & 16-20 & all & 0-19& 19-20& all & 0-15 & 16-20 & all \\
    \hline
    \hline
     ILT~\cite{michieli2019incremental}&- & - & - &  3.7&  5.7&  4.2&  69.1&  16.4&  66.4&63.2&  39.5&57.3\\
 MiB~\cite{cermelli2020modeling}& 9.5& 4.1& 6.9& 35.1& 13.5 & 29.7& 69.6& 25.6& 67.4&71.8& 43.3&64.7\\
 PLOP~\cite{douillard2021plop}& 9.7& 7.0& 8.4& 57.8& 13.6& 46.4& 75.3& \textbf{38.8}& 73.6& 71.0& 42.8&64.2\\
     SSUL~\cite{cha2021ssul}& 65.4& 34.9& 50.8& 73.9& 32.1& 64.0& 77.3& 22.4& 74.7& 76.4& 45.6&69.1\\
     % DKD&73.10 &46.51 &60.44 &76.34 &39.3 & 67.54& 69.57&53.52 &58.10 &58.70&47.74& 49.30& 77.56&54.13 & 71.98\\
 MicroSeg~\cite{zhang2022mining}& -& -& -& 73.7& 24.1& 61.9& \bf{80.6}& 16.0&\bf{77.4} & 77.4& 43.4&69.3\\
 RCIL~\cite{zhang2022representation}& 30.6& 4.7& 18.2& 66.1& 18.2& 54.7& -& -& -& 75.0& 42.8&67.3\\
     % EWF& & & & & & & & & & & &\\
     % TIKP& &&& &&&&&&&&\\ 
    \hline
     {\bf Ours}& {\bf 59.3}&{\bf 43.6}& {\bf 51.8}& {\bf 76.9}& {\bf 46.0}& {\bf 69.6}&77.3&36.8& 75.4&{\bf 77.9}&{\bf 53.0}&{\bf 72.0}\\
    \hline
     joint&78.4 & 76.4&77.4&79.8 & 72.4&77.4& 77.5 & 77.0 &77.4&79.7 & 72.4 &77.4\\
    \Xhline{1.3pt}
    \end{tabular}
    \label{table1}
    \label{tab: VOC}
    \vspace{-0.05in}
\end{table*}

\begin{table*}[t!]
    \centering

    \caption{Detailed experimental results of Pascal VOC 2012 with class using Resnet101}
    \vspace{-0.1in}
    \begin{tabular}{c|ccccccccccccccccccccc|c}
    \Xhline{1.3pt}
    \textbf{Method} & bg & acro & bike & bird&boat & bott & bus & car & cat & cha. & cow & table & dog & hrs. & mbik & pers. & plnt &sleep & sofa & train & tv & mIoU\\
    % \multicolumn{1}{c|}{} & 0-10 & 11-20 & all & 0-15 & 16-20 & all & 0-5 & 6-20 & all & 0-2& 3-20& all & 0-15 & 16-20 & all \\
    \hline
    \hline
     10-1 (11)& 86.0&86.9&38.5&84.4&64.0&78.6&85.6&87.6&87.5&22.6&68.7&45.6&78.8&63.4&75.1&80.4&33.0&66.4&25.9&62.3&49.8&65.3\\
 2-2 (10)&83.5&83.4&38.0&70.2&61.1&47.5&78.8&58.9&83.8&4.5&44.5&50.9&74.7&49.4&72.6&50.5&40.6&59.9&26.1&63.9&52.1&56.9 \\
% 15-1 (6)& 87.0&88.6&39.8&87.6&71.3&80.6&92.1&89.8&92.8&37.0&82.7&61.1&89.0&83.8&82.3&86.1&40.5&75.8&24.5&59.8&38.2&70.1\\
     5-3 (6)& 88.2&88.8&37.2&87.0&67.2&79.3&77.7&83.6&83.0&19.9&62.0&54.5&77.4&63.2&76.7&82.8&41.6&72.5&29.8&69.6&52.6&66.4\\
     % DKD&73.10 &46.51 &60.44 &76.34 &39.3 & 67.54& 69.57&53.52 &58.10 &58.70&47.74& 49.30& 77.56&54.13 & 71.98\\
 15-5 (2)& 90.4&89.8&40.9&90.5&71.9&81.4&91.7&90.0&93.1&36.3&85.0&59.8&89.3&84.6&84.3&86.6&37.8&76.4&32.0&83.1&62.6&74.2\\
    \Xhline{1.3pt}
    \end{tabular}
    \label{table2}
    \label{tab: VOC_class}
    \vspace{-0.05in}
\end{table*}

%\vspace{-0.2in}
\begin{figure}[t]
    % \caption{mIoU on VOC 5-3 with different instance number.}
    \centering
    \includegraphics[width=1\linewidth]{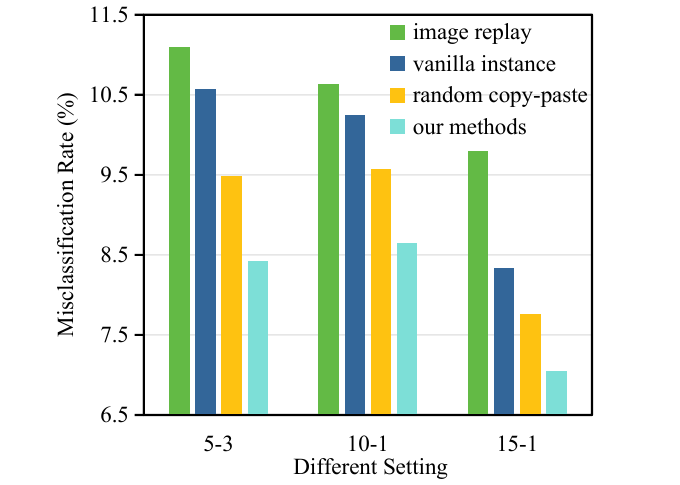}
   % \vspace{-0.15in}
     \caption{Background Misclassification Rate on different setting.}
    \label{fig: background-shift}
    \vspace{-0.15in}
\end{figure} 

\subsection{Analysis of the Background Shift problem}

Our method fuses instances into the background of new data, which mitigates the background shift problem by replacing confusing background information with accurately labeled instances. To further validate the effectiveness of our approach, we conducte experiments where we calculate the proportion of pixels from the target classes that are misclassified as background—an indicator of the background shift problem. As shown in the Figure~\ref{fig: background-shift}, our method is compared with the traditional image replay method, the vanilla instance replay method, and the random copy-pasting method. The results demonstrate that our method is more effective in addressing the background shift issue compared to the others.

\subsection{Analysis on the Effectiveness of EIR }
% to fairly evaluate the effectiveness of instance replay. it would be beneficial to apply it to previous replay-based methods. such as SSUL-M

% Analysis on the Effectiveness of EIR 
We conducted experiments while maintaining all other experimental conditions consistent with past Image Replay work Microseg-M~\cite{zhang2022mining}, with the sole exception of substituting Image Replay with EIR to more fairly and comprehensively evaluate the effectiveness of our proposed Enhanced Instance Replay (EIR) method against the traditional Image Replay approach. Results in Table~\ref{tab: contrast} unequivocally show EIR's superiority and compatibility with CSS settings. Under each setting, EIR consistently outperforms Image Replay. Notably, EIR's memory size was significantly lower, requiring only 16MB compared to Image Replay's 60MB, highlighting Enhanced Instance Replay's advantages.

% %这一部分其实可以不用写了，因为已经有 vanilla instance replay了，所以这部分暂时先不写了
% % 标题可以再写一下！！ 11-18
% % 11-19 将这部分写好。 还有background shift的描述
% \subsection{Analysis the different method of instance replay}
% % 更加一步证明了为什么不将instance单独输入模型训练
% % 还有一个instance 的消融实验
% % 【1】旧类图像+新类图像
% % 【2】旧类图像+新类instance，新类往旧类图像上贴
% % 【3】旧类instance+新类instance
% % 【4】旧类instance+新类图像，旧类往新类图像上贴

\subsection{Comprehensive Experimental Results}
In this section, we present the results on Pascal VOC 2012 of the disjoint setting and detailed results of Pascal VOC 2012 5-3 overlapped setting with class.

\noindent
{\bf The experimental result on disjoint setting.~~}As shown in Table~\ref{tab: VOC}, we present the experimental results of disjoint setting for a fair comparison with prior works. In the disjoint setting, images do not contain future classes, making it less challenging and realistic compared to the overlapped setting. The result shows that our methods demonstrates significant advantages over other methods.

\noindent
{\bf The details of experimental results of Pascal VOC 2012.~~}
As shown in the Table~\ref{tab: VOC_class}, we also present the results of Pascal VOC 2012 overlapped setting with each class. The results demonstrate that even in long setting, our method maintains strong performance across all classes.

\section{More Visual Results}
We present additional visual results for Pascal VOC 2012 and ADE 20K in Figure~\ref{fig: voc_visual}, and~\ref{fig: ade_visual} at the end of the supplementary material. These visual illustrations showcase the high-quality outputs generated by our segmentation network.

% \section{Code Segment}
% In this section, we provide an anonymous link showcasing the core components of our code, allowing you to explore and understand the details of our method: \href{https://github.com/paperid-12517/EIR}{https://github.com/paperid-12517/EIR}.

\begin{figure*}[t!]
    \centering
    \includegraphics[width=1\linewidth]{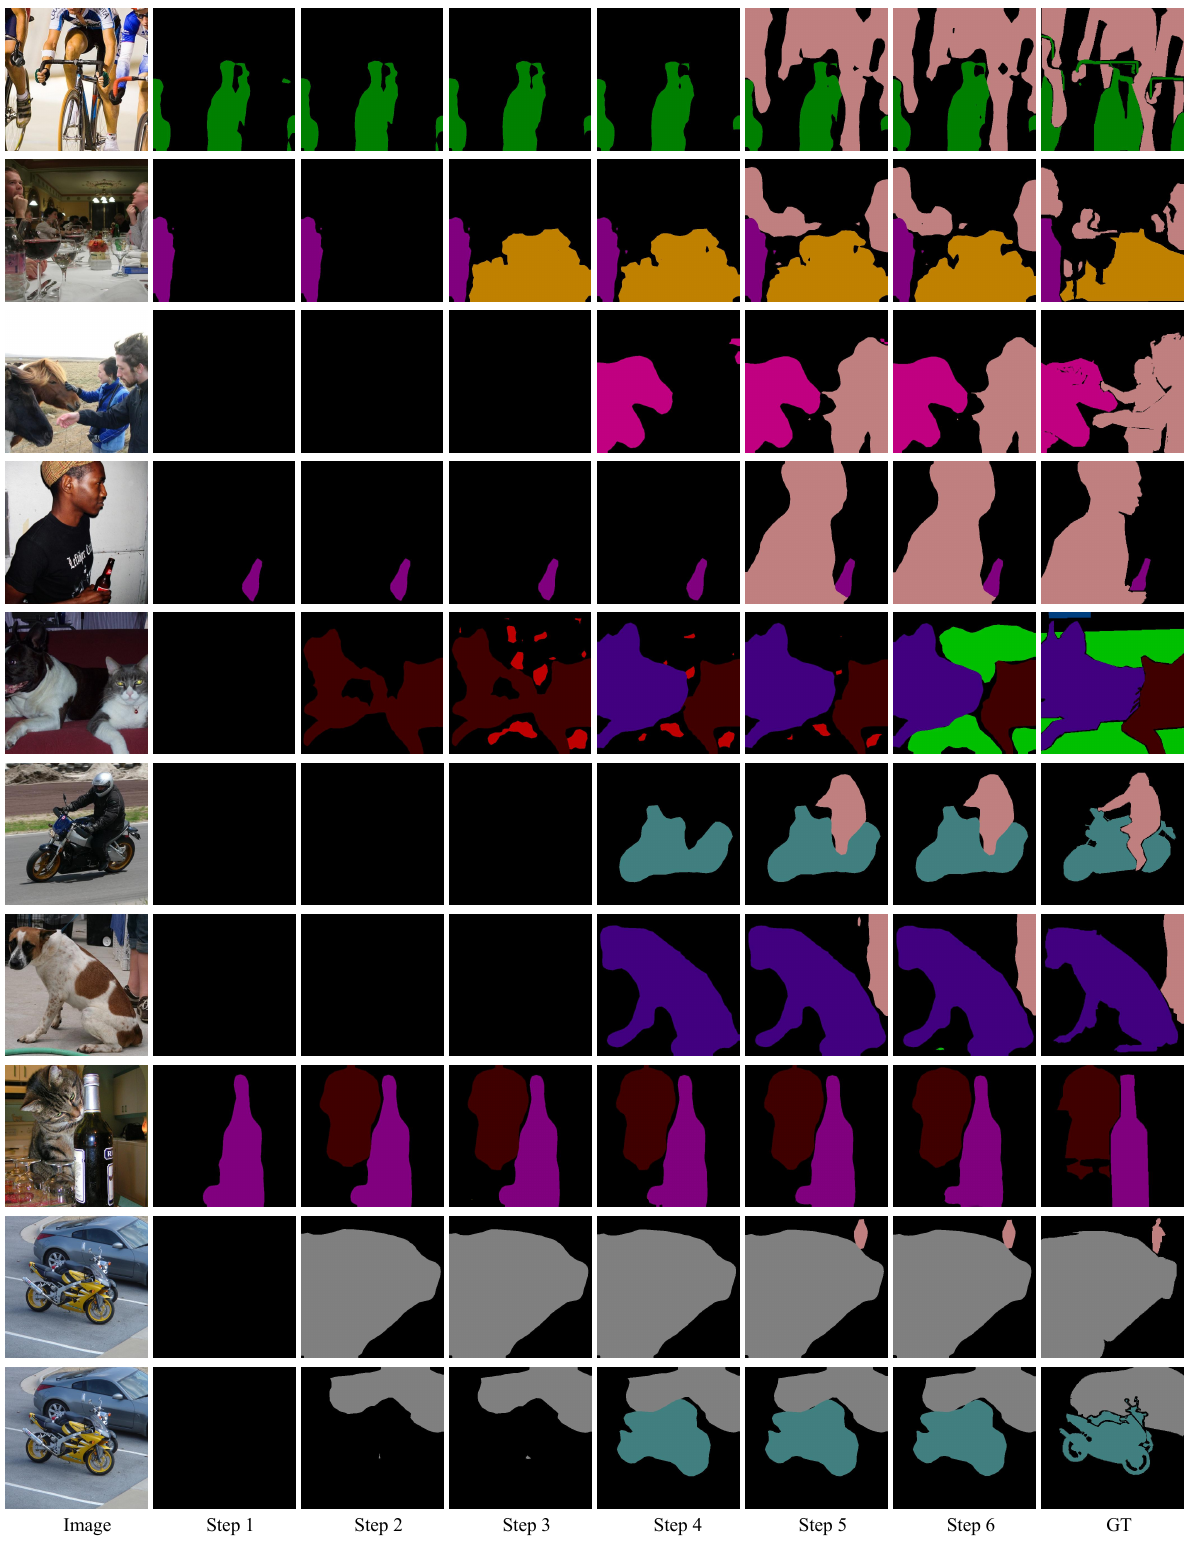}
    \vspace{-0.4in}
    \caption{Segmentation results on Psacal VOC 2012 between our methods in different steps.}
    % \vspace{-1.0in}
    \label{fig: voc_visual}
\end{figure*}
 \vspace{-1.0in}

\vspace{-1.0in}
\begin{figure*}[t!]
    \centering
    \includegraphics[width=1\linewidth]{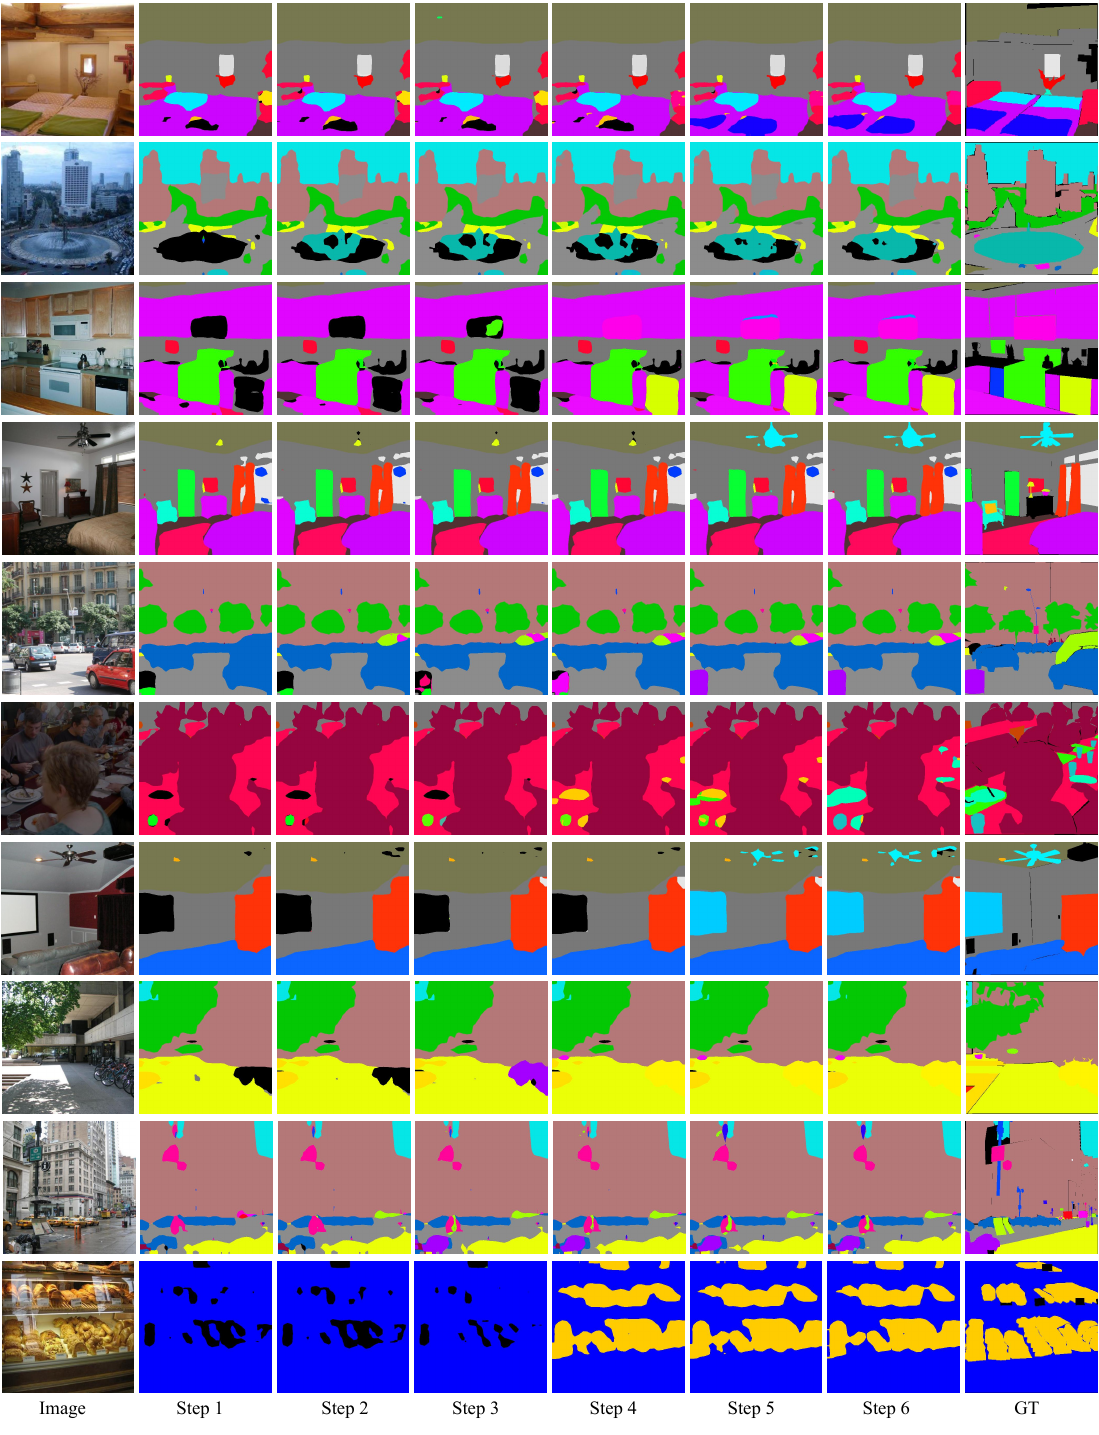}
    \vspace{-0.3in}
    \caption{Segmentation results on ADE 20K between our methods in different steps.}
    \label{fig: ade_visual}
\end{figure*}
\vspace{-1.0in}
% \section{Limitation}
